# Supplementary material for: PlanGPT: Enhancing Urban Planning with Tailored Language Model and Efficient Retrieval
Source: arXiv:2402.19273 source file (2024-02-29)
Supplement: Supplementary file 1 [file baichuan-13b-chat.tex]

\textbf{Baichuan2-13B-Chat}:\\
\hline
\textbf{Prompt}:\\
\begin{CJK*}{UTF8}{gbsn}
假设你是一个善于写中国城乡规划文本的工作人员, 请你根据 \#城乡规划文本特征\# 将以下 \#原文\# 改写成符合城乡规划风格的文字。\\
\#城乡规划文本特征\#：\\
1. 文字连贯，内容完整。\\
2. 用语规范，内容官方严谨，不使用口语化的表达方式，不出现英文、拼音、网络用语等。\\
3. 符合政府文件风格, 语言优美, 内容充实, 不出现概念堆叠与重复内容。\\
\#原文\#：\\
这份规划是庆安县国土空间的全面规划，旨在指导各类开发建设活动，保护土地资源，规划国土空间，管理空间发展。该规划是根据国家和省级工作安排，结合庆安县实际情况制定的文件。在规划中考虑了庆安县的资源环境承载能力和国土空间开发适宜性，评估了现有国土空间开发保护情况，明确了全县国土空间的资源特征和目标。我们的目标是积极落实国家、省、市级要求，与重大区域战略协同发展。规划还包括优化三类空间布局、明确控制线、划分规划分区及用途分类、加强自然和人文资源保护利用，提升国土空间品质，完善基础支撑体系，制定国土空间整治和生态修复任务，优化中心城区空间布局，明确发展方向，提出规划传导指引和近期建设计划，完善规划实施保障机制，为庆安建设更加富强、民主、和谐、美丽的社会主义现代化新庆安提供国土空间保障。\\
\#城乡规划风格文字\#\\
\end{CJK*}
\textbf{Response}:\\
\begin{CJK*}{UTF8}{gbsn}
关于庆安县国土空间规划的编制说明\\    本次编制的庆安县国土空间总体规划，旨在全面规范和指导区域内各类开发建设项目。规划严格遵循国家及省级工作安排，紧密结合庆安县实际，综合考量本县土地资源禀赋与国土空间开发潜力，对现有开发保护状况进行全面评估，并确定土地资源特征及规划目标。\\   规划强调落实国家、省、市相关规划要求，与区域重大战略协同并进。同时，规划内容涉及三类空间布局优化、管控边界划定、功能分区及用途分类明确、自然与文化遗产保护强化、国土空间品质提升、基础支撑体系完善以及国土空间整治和生态修复任务。此外，规划明确了中心城区发展策略，规划传导机制，及近期建设计划，并设置了规划实施保障体系，以确保庆安县在社会主义现代化建设中，实现富强、民主、和谐、美丽的目标。\\   本规划将对庆安县国土空间进行科学规划和有效管理，促进区域可持续发展，为庆安县构建现代化国土空间布局提供坚实保障。
\end{CJK*}
