# Supplementary material for: PlanGPT: Enhancing Urban Planning with Tailored Language Model and Efficient Retrieval
Source: arXiv:2402.19273 source file (2024-02-29)
Supplement: Supplementary file 2 [file chatglm-2shots.tex]

\textbf{ChatGLM-2shots}:\\
\hline
\textbf{Prompt}:\\
\begin{CJK*}{UTF8}{gbsn}
假设你是一个善于写中国城乡规划文本的工作人员, 请你根据 \#城乡规划文本特征\# 将以下 \#原文\# 改写成符合城乡规划风格的文字。\\
\#城乡规划文本特征\#：\\
1. 文字连贯，内容完整。\\
2. 用语规范，内容官方严谨，不使用口语化的表达方式，不出现英文、拼音、网络用语等。\\
3. 符合政府文件风格, 语言优美, 内容充实, 不出现概念堆叠与重复内容。\\
\#样例1\#:\\
兰溪市位于浙江省中西部，地处钱塘江中游，金衢盆地北缘。兰溪建县近一千四百年，历史悠久、人才辈出，是浙江省历史文化名城。兰溪自古物华天宝、商贸繁荣，有“三江之汇、七省通衢”之美誉，创造了“天下江南”“钱塘第一商埠”“民国第一县”“全国工业学兰溪”的辉煌。1985年撤县建市以来，兰溪已发展成为有一定旅游知名度的典型工业城市。建立国土空间规划体系并监督实施是生态文明背景下党中央做出的重大决策部署,是国家治理体系和治理能力现代化的重要组成部分。按照自然资源部、浙江省政府的统一工作安排，紧扣“实干争先、再创辉煌”目标要求，奋力实施“智造立市、拥江兴市、环境活市、共富强市”发展战略，兰溪市人民政府组织编制了《兰溪市国土空间总体规划（2021-2035年）》（以下简称规划）。规划是对《浙江省国土空间规划（2021-2035年）》、《金华市国土空间总体规划（2021-2035年）》的细化落实。规划同时是兰溪市未来国土空间保护、开发、利用、修复的行动纲领，是贯彻新发展理念的空间蓝图，也是兰溪市编制各乡镇国土空间总体规划和详细规划的基本依据，对相关专项规划具有战略引领和约束作用。本文件为规划草案概要，规划所有图纸、数据以最终批复版为准。本文件部分照片来自网络，如涉及版权问题，请与兰溪市自然资源和规划局联系。\\
\#样例2\#:\\
建立国土空间规划体系并监督实施，是党中央、国务院做出的重大部署。《什邡市国土空间总体规划（2021-2035年）》，将是什邡未来到2035年各类开发保护建设活动的基本依据。把握新发展机遇，贯彻新发展理念，融入新发展格局，以推动高质量发展为主题，以满足人民日益增长的美好生活需要为根本目的，本轮国土空间总体规划确定了新时期什邡的目标定位、发展战略和各类空间布局。目前，什邡市国土空间总体规划已形成草案，为了让公众充分了解规划内容，凝聚社会共识，征询公众意见，现进行草案公示。\\
\#原文\#：\\
这份规划是庆安县国土空间的全面规划，旨在指导各类开发建设活动，保护土地资源，规划国土空间，管理空间发展。该规划是根据国家和省级工作安排，结合庆安县实际情况制定的文件。在规划中考虑了庆安县的资源环境承载能力和国土空间开发适宜性，评估了现有国土空间开发保护情况，明确了全县国土空间的资源特征和目标。我们的目标是积极落实国家、省、市级要求，与重大区域战略协同发展。规划还包括优化三类空间布局、明确控制线、划分规划分区及用途分类、加强自然和人文资源保护利用，提升国土空间品质，完善基础支撑体系，制定国土空间整治和生态修复任务，优化中心城区空间布局，明确发展方向，提出规划传导指引和近期建设计划，完善规划实施保障机制，为庆安建设更加富强、民主、和谐、美丽的社会主义现代化新庆安提供国土空间保障。\\
\#城乡规划风格文字\#\\
\end{CJK*}
\textbf{Response}:\\
\begin{CJK*}{UTF8}{gbsn}
本规划值为庆安县国土空间全面规划，旨在引导各类开发建设活动，维护土地资源，规划国土空间使用，并进行空间发展管理。该规划是根据国家和省级的工作要求，结合庆安县的实际情况制定的。在规划中，我们考虑了庆安县的资源环境承载能力和国土空间开发适宜性，评估了现有的国土空间开发保护情况，明确了全县国土空间的资源特征和目标。我们的目标是积极执行国家、省、市级的工作要求，与重大区域战略协同发展。规划包括了优化三类空间布局、明确控制线、划分规划分区及用途分类、加强自然和人文资源保护利用，提升国土空间品质，完善基础支撑体系，制定国土空间整治和生态修复任务，优化中心城区空间布局，明确发展方向，提出规划传导指引和近期建设计划，完善规划实施保障机制，为庆安建设更加富强、民主、和谐、美丽的社会主义现代化新庆安提供国土空间保障。
\end{CJK*}
