# Supplementary material for: PlanGPT: Enhancing Urban Planning with Tailored Language Model and Efficient Retrieval
Source: arXiv:2402.19273 source file (2024-02-29)
Supplement: Supplementary file 3 [file chatglm.tex]

\textbf{ChatGLM}:\\
\hline
\textbf{Prompt}:\\
\begin{CJK*}{UTF8}{gbsn}
假设你是一个善于写中国城乡规划文本的工作人员, 请你根据 \#城乡规划文本特征\# 将以下 \#原文\# 改写成符合城乡规划风格的文字。\\
\#城乡规划文本特征\#：\\
1. 文字连贯，内容完整。\\
2. 用语规范，内容官方严谨，不使用口语化的表达方式，不出现英文、拼音、网络用语等。\\
3. 符合政府文件风格, 语言优美, 内容充实, 不出现概念堆叠与重复内容。\\
\#原文\#：\\
这份规划是庆安县国土空间的全面规划，旨在指导各类开发建设活动，保护土地资源，规划国土空间，管理空间发展。该规划是根据国家和省级工作安排，结合庆安县实际情况制定的文件。在规划中考虑了庆安县的资源环境承载能力和国土空间开发适宜性，评估了现有国土空间开发保护情况，明确了全县国土空间的资源特征和目标。我们的目标是积极落实国家、省、市级要求，与重大区域战略协同发展。规划还包括优化三类空间布局、明确控制线、划分规划分区及用途分类、加强自然和人文资源保护利用，提升国土空间品质，完善基础支撑体系，制定国土空间整治和生态修复任务，优化中心城区空间布局，明确发展方向，提出规划传导指引和近期建设计划，完善规划实施保障机制，为庆安建设更加富强、民主、和谐、美丽的社会主义现代化新庆安提供国土空间保障。\\
\#城乡规划风格文字\#\\
\end{CJK*}
\textbf{Response}:\\
\begin{CJK*}{UTF8}{gbsn}
本规划值为庆安县国土空间全面规划，旨在引导各类开发建设活动，维护土地资源，规划国土空间使用，并进行空间发展管理。该规划是根据国家和省级的工作要求，结合庆安县的实际情况制定的。在规划中，我们考虑了庆安县的资源环境承载能力和国土空间开发适宜性，评估了现有的国土空间开发保护情况，明确了全县国土空间的资源特征和目标。我们的目标是积极执行国家、省、市级的工作要求，与重大区域战略协同发展。规划包括了优化三类空间布局、明确控制线、划分规划分区及用途分类、加强自然和人文资源保护利用，提升国土空间品质，完善基础支撑体系，制定国土空间整治和生态修复任务，优化中心城区空间布局，明确发展方向，提出规划传导指引和近期建设计划，完善规划实施保障机制，为庆安建设更加富强、民主、和谐、美丽的社会主义现代化新庆安提供国土空间保障。
\end{CJK*}
