# Supplementary material for: PlanGPT: Enhancing Urban Planning with Tailored Language Model and Efficient Retrieval
Source: arXiv:2402.19273 source file (2024-02-29)
Supplement: Supplementary file 4 [file gpt35.tex]

\textbf{GPT-3.5-turbo}:\\
\hline
\textbf{Prompt}:\\
\begin{CJK*}{UTF8}{gbsn}
假设你是一个善于写中国城乡规划文本的工作人员, 请你根据 \#城乡规划文本特征\# 将以下 \#原文\# 改写成符合城乡规划风格的文字。\\
\#城乡规划文本特征\#：\\
1. 文字连贯，内容完整。\\
2. 用语规范，内容官方严谨，不使用口语化的表达方式，不出现英文、拼音、网络用语等。\\
3. 符合政府文件风格, 语言优美, 内容充实, 不出现概念堆叠与重复内容。\\
\#原文\#：\\
这份规划是庆安县国土空间的全面规划，旨在指导各类开发建设活动，保护土地资源，规划国土空间，管理空间发展。该规划是根据国家和省级工作安排，结合庆安县实际情况制定的文件。在规划中考虑了庆安县的资源环境承载能力和国土空间开发适宜性，评估了现有国土空间开发保护情况，明确了全县国土空间的资源特征和目标。我们的目标是积极落实国家、省、市级要求，与重大区域战略协同发展。规划还包括优化三类空间布局、明确控制线、划分规划分区及用途分类、加强自然和人文资源保护利用，提升国土空间品质，完善基础支撑体系，制定国土空间整治和生态修复任务，优化中心城区空间布局，明确发展方向，提出规划传导指引和近期建设计划，完善规划实施保障机制，为庆安建设更加富强、民主、和谐、美丽的社会主义现代化新庆安提供国土空间保障。\\
\#城乡规划风格文字\#\\
\end{CJK*}
\textbf{Response}:\\
\begin{CJK*}{UTF8}{gbsn}
本文件为庆安县的综合规划，主要目的是为了指导各类开发建设活动，保护土地资源，规划国土空间，管理空间发展。该规划是根据国家和省级工作安排，并结合庆安县的实际情况制定的文件。在规划过程中充分考虑了庆安县的资源环境承载能力以及国土空间开发适宜性，并评估了现有国土空间开发保护情况，明确了全县国土空间的资源特征和目标。我们的目标是积极践行国家、省、市级要求，并与重大区域战略协同发展。规划内容还包括优化三类空间布局、明确控制线、划分规划分区及用途分类、加强自然和人文资源的保护利用，提升国土空间品质，完善基础支撑体系，制定国土空间整治和生态修复任务，优化中心城区空间布局，明确发展方向，提出规划传导指引和近期建设计划，完善规划实施保障机制，为庆安县建设更加富强、民主、和谐、美丽的社会主义现代化新庆安提供国土空间保障。
\end{CJK*}
